# Supplementary material for: Phonon Quantum Phase Transition
Source: arXiv:1809.06495 source file (2018-09-18)
Supplement: Supplementary file 1 [file supplementary_text.tex]

\section{Renormalization Group Scaling Equations}

In this part we show how the action, Eq.~\ref{action},  in the main text is affected by the rescaling  procedure.  Here we use  $k'=bk$ which corresponds to the rescaling $R'=R/b$ in real space. Then, we have after rescaling the following action 

\begin{equation}
\begin{split}
 S[\phi^{s}]&= \sum_{n,0<\textbf{k} \leq \Lambda/b} \overline{\phi}_{n\textbf{k}}^{s} \left( -i\omega_{n} + \omega_\textbf{k} - \frac{n_{dis} \Delta_\textbf{k}}{\omega_\textbf{k}} \right) \phi_{n\textbf{k}}^{s}
 + \frac{g}{4!} \int_{0}^{\beta} d\tau   \int d^{D} R \phi^{4,s} (R, \tau)\\
% &=\sum_{n,0<\textbf{k}\leq \Lambda/b} \overline{\phi}_{n\textbf{k}}^{'s} \left( -i\omega_{n}^{'}b^{-2y_{\phi}-z} + \omega_{\textbf{k}}^{'}b^{-2y_{\phi}-z_{0}} - b^{z_{0}-2y_{\phi}-2} \frac{n_{dis}' \Delta_{\textbf{k}}}{\omega_\textbf{k}^{'}} \right) \phi_{n\textbf{k}}^{'s}
% +\frac{g}{4!} b^{z_{0}-D} \int_{0}^{\beta} d\tau^{'}   \int d^{D} R^{'} \phi^{4,s} (R^{'}, \tau^{'}). 
 \end{split}
\end{equation}

The requirement that the rescaled action is equivalent to the original one yields the scaling relations 

\begin{equation}
\begin{aligned}
& \omega_{\textbf{k}}'=\omega_{\textbf{k}}b^{z_{0}} \qquad \omega_{n}'=b^{z}\omega_{n} \qquad n_\text{dis}'=b^2 n_\text{dis} \qquad  \tau'=b^{-z_{0}} \tau \\
& \phi_{n\textbf{k}}^{s'}=b^{y_{\phi}} \phi_{n\textbf{k}}^s \qquad \phi(\textbf{R}',\tau') = b^{D/2}\phi(\textbf{R},\tau) \qquad  T'=b^{z}T 
\end{aligned}
\end{equation}

where we have imposed scale invariance on the action to obtain:
\begin{equation}
-2y_{\phi}-z_{0}=0 \qquad -2y_{\phi}-z=0 \qquad z_{0}-2y_{\phi}-2=0
\end{equation}

\begin{equation}\label{newescaling}
\Delta_{\textbf{k}}'=b^{z_{0}-2y_{\phi}-2} \Delta_{\textbf{k}}= b^{2z_{0}-2} \Delta_{\textbf{k}}; \qquad g'=  b^{z_{0}-D}g
\end{equation}

In the rest of the paper, we will consider $b=e^l$ with $l$ being a small value.
